# Supplementary material for: Identity Decoupling for Multi-Subject Personalization of Text-to-Image Models
Source: arXiv:2404.04243 source file (2024-10-28)
Supplement: Supplementary file 1 [file appendix_sd2_qual.pdf]

Refs

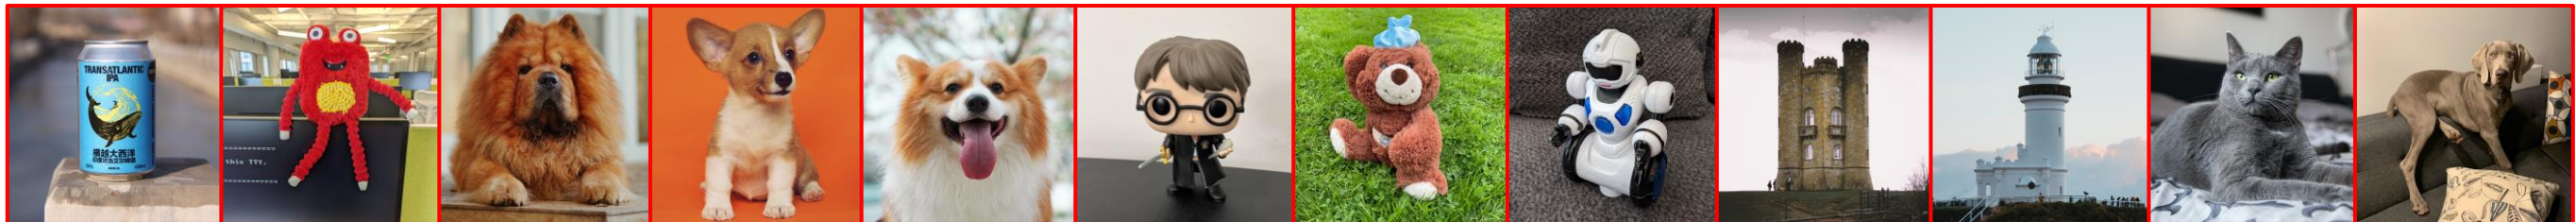

Custom Diffusion

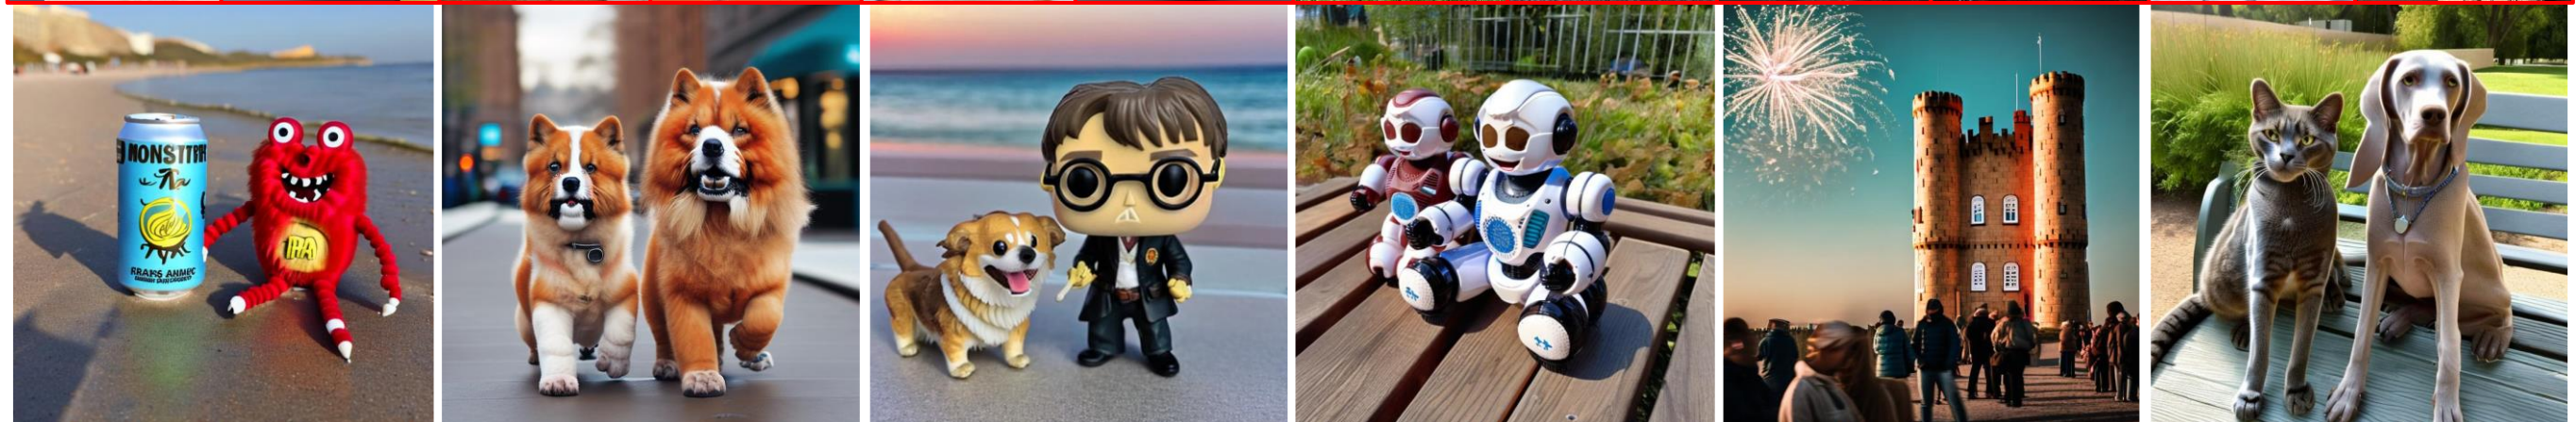

Cones2

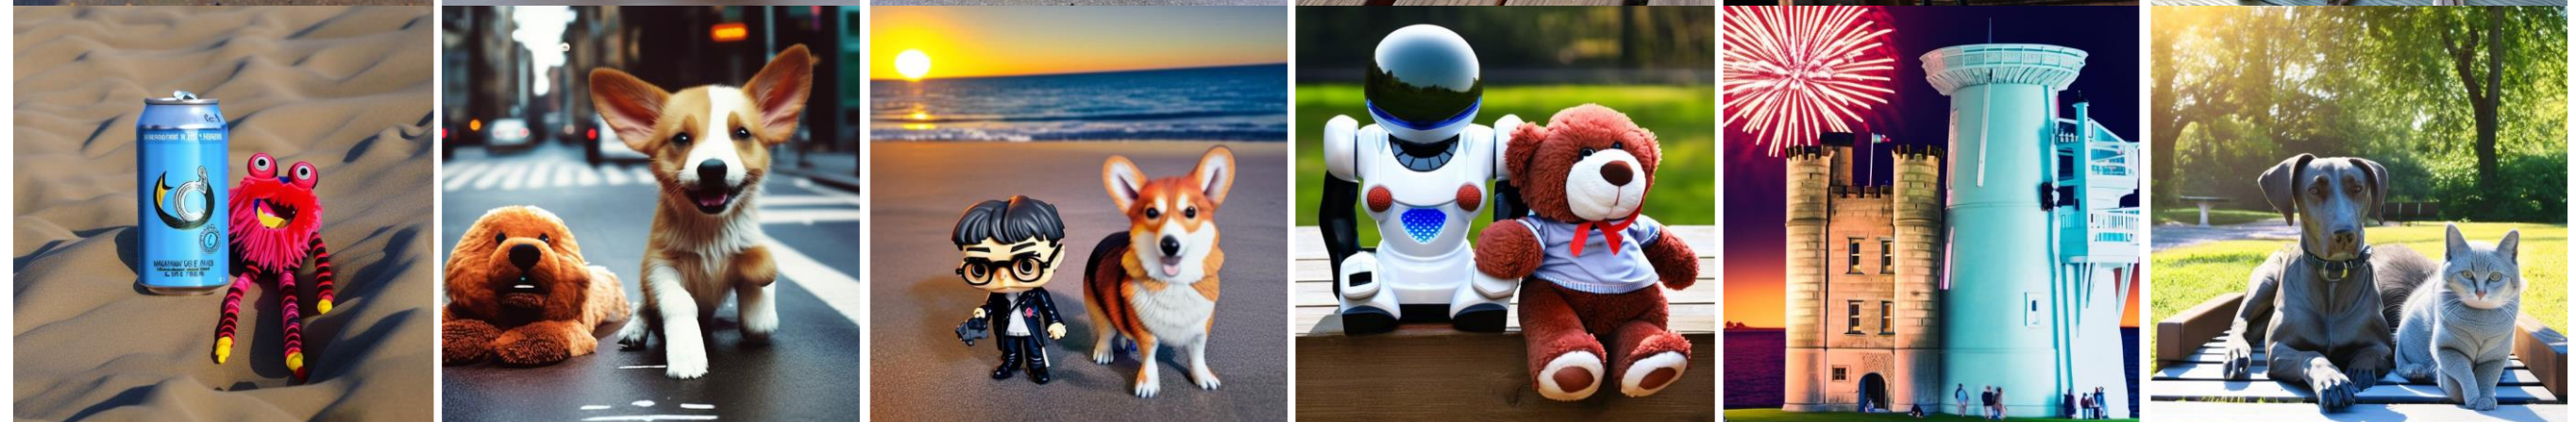

Mix-of-Show

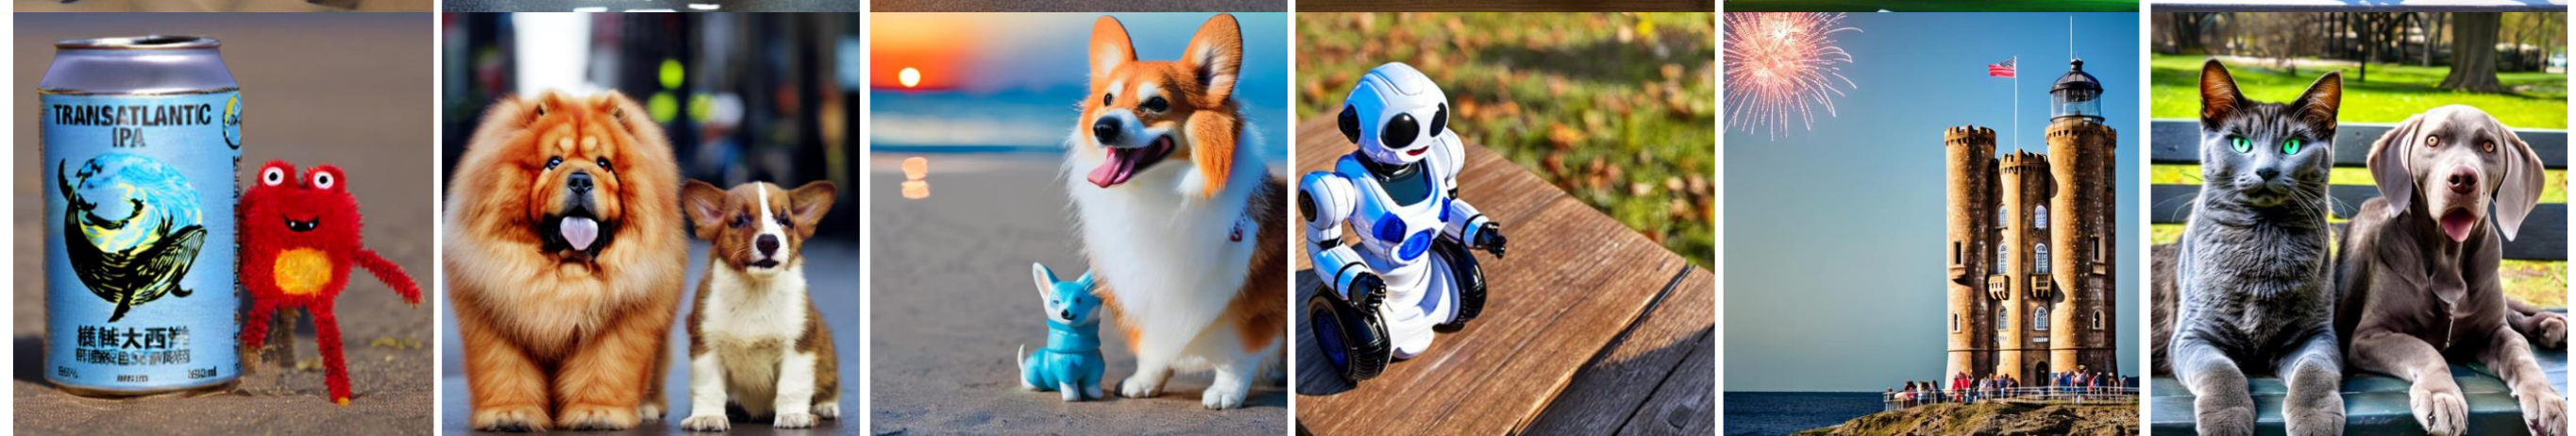

MuDI (Ours)

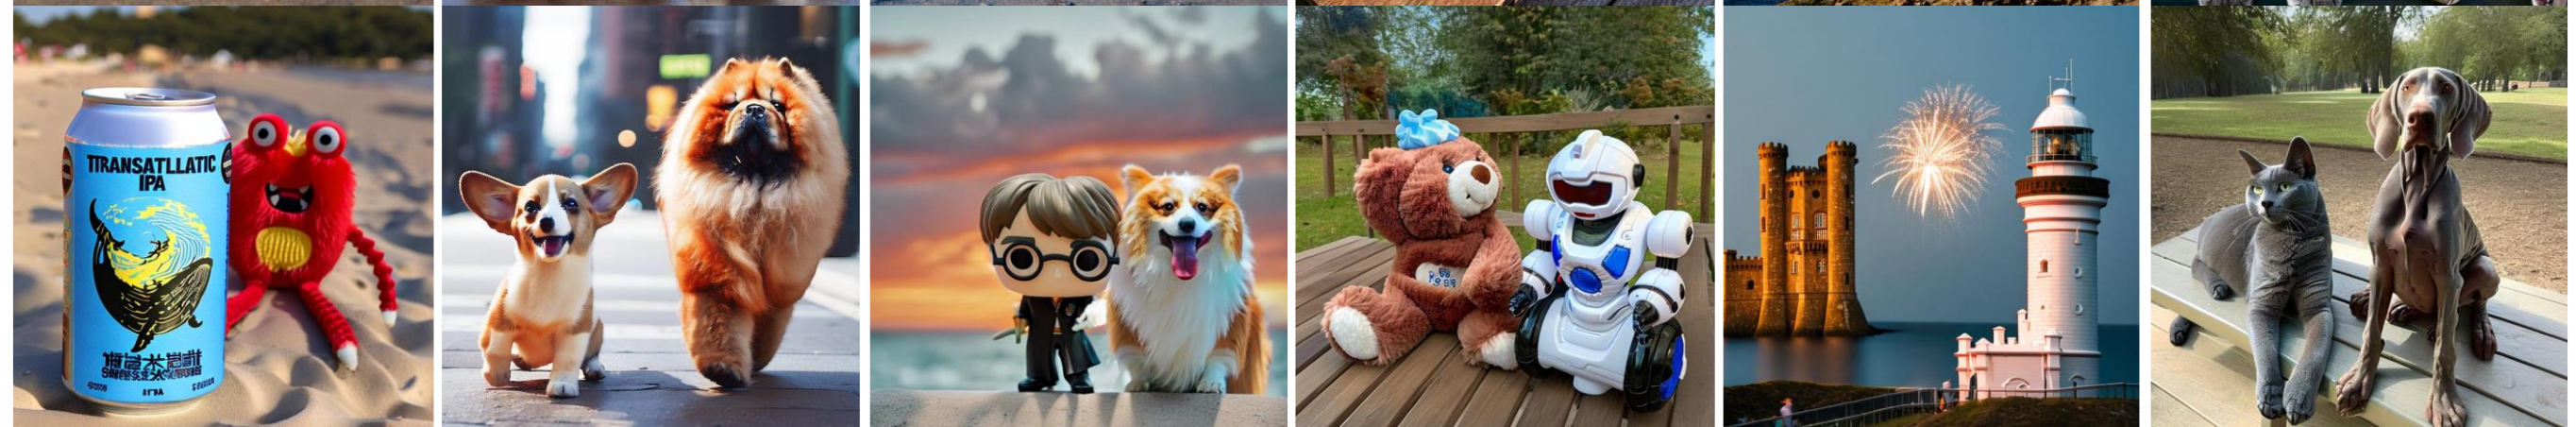

*"... at the beach under a bright sun."*

*"... walking in a bustling city street corner."*

*"... watching a beautiful sunset at the beach."*

*"... on a wooden bench in a sunny park."*

*"..., people watching fireworks."*

*"... resting on a bench in a sunny park."*
